# Supplementary material for: Visual Monitoring for Multiple Points of Interest on a 2.5D Terrain using a UAV with Limited Field-of-View Constraint
Source: arXiv:1903.07363 source file (2019-03-18)
Supplement: Supplementary file 1 [file appendix.tex]

\appendix{\textbf{Horizon Computation:}\label{app:horizonComp}
Stewart's method \cite{horizonComputation} computes an approximation of the global horizon. It divides the angular space into $k$ sectors and computes a constant horizon value for each sector. To compute the elevation angle for a particular sector a coordinate transformation is performed to align the new axes with the a $(\pi/2)$ clockwise rotation of sector boundaries. In the new non-orthogonal coordinate system, all points on the terrain with a smaller value for the x-coordinate and a larger value for the y-coordinate than the point under consideration (viewpoint) lie in the sector and must be considered to compute the maximum sectoral elevation. If processed in the increasing order of x-coordinate value, all points in the sector are processed before the viewpoint. This makes it easy to consider all points in a sector and find the maximum elevation angle. The maximum elevation angle amongst all points that lie in a sectoral space when observed from a viewpoint, is used as an approximation for the elevation angle for the entire sector. This is repeated over all sectors to compute the maximum elevation (read global horizon). The elevation in turn is used to compute the visibility angle for each direction for all points of interest. The number of sectors, $k$, is a use defined parameter. The value of $k$ affects the accuracy of the approximate horizon computation method. Narrow sectors (large $k$ value) can miss terrain features and underestimate the elevation, while broad sectors (small value of $k$) could lead to unwanted over estimation. The interested reader may refer \cite{horizonComputation} for more involved details on the algorithm.
